# Supplementary material for: Broken-symmetry self-consistent GW approach: degree of spin contamination and evaluation of effective exchange couplings in solid antiferromagnets
Source: arXiv:2207.12064 source file (2022-07-25)
Supplement: Supplementary file 1 [file SI.pdf]

# Broken-symmetry self-consistent GW approach: degree of spin contamination and evaluation of effective exchange couplings in solid antiferromagnets

Pavel Pokhilko[1] and Dominika Zgid[1,2]

[1]*Department of Chemistry, University of Michigan, Ann Arbor, Michigan 48109, USA*

[2]*Department of Physics, University of Michigan, Ann Arbor, Michigan 48109, USA*

## 1. SPIN CORRELATORS

TABLE S1: $SS_{AB}^{\mathbf{k}=0}$, computed for the NiO **cell 1** with UHF.

| | Ni | O | Ni | O |
|---|---|---|---|---|
| Ni | -0.401 | 0.159 | 1.657 | 0.154 |
| O | 0.159 | 0.328 | 0.154 | 0.095 |
| Ni | 1.657 | 0.154 | -0.401 | 0.159 |
| O | 0.154 | 0.095 | 0.159 | 0.328 |

TABLE S2: $SS_{AB}^{\mathbf{k}=0}$, computed for the NiO **cell 1** with GW.

| | Ni | O | Ni | O |
|---|---|---|---|---|
| Ni | 0.269 | 0.336 | 2.581 | 0.481 |
| O | 0.336 | 0.874 | 0.481 | 0.244 |
| Ni | 2.581 | 0.481 | 0.269 | 0.336 |
| O | 0.481 | 0.244 | 0.336 | 0.874 |

TABLE S3: $SS_{AB}$, computed for the NiO **cell 1** with UHF.

| | Ni | O | Ni | O |
|---|---|---|---|---|
| Ni | 0.037 | 0.106 | 1.885 | 0.199 |
| O | 0.106 | 0.014 | 0.199 | 0.041 |
| Ni | 1.885 | 0.199 | 0.037 | 0.106 |
| O | 0.199 | 0.041 | 0.106 | 0.014 |

TABLE S4: $SS_{AB}$, computed for the NiO **cell 1** with GW.

| | Ni | O | Ni | O |
|---|---|---|---|---|
| Ni | 0.193 | 0.179 | 2.147 | 0.355 |
| O | 0.179 | 0.109 | 0.355 | 0.094 |
| Ni | 2.147 | 0.355 | 0.193 | 0.179 |
| O | 0.355 | 0.094 | 0.179 | 0.109 |

TABLE S5: $SS_{AB}^{\mathbf{k}=0}$, computed for the NiO **cell 2** with UHF.

| | Ni | O | Ni | O |
|---|---|---|---|---|
| Ni | 1.549 | 0.101 | 3.280 | 0.101 |
| O | 0.101 | 0.054 | 0.101 | 0.008 |
| Ni | 3.280 | 0.101 | 1.549 | 0.101 |
| O | 0.101 | 0.008 | 0.101 | 0.054 |

TABLE S6: $SS_{AB}^{\mathbf{k}=0}$, computed for the NiO **cell 2** with GW.

| | Ni | O | Ni | O |
|---|---|---|---|---|
| Ni | 1.989 | 0.170 | 3.337 | 0.170 |
| O | 0.170 | 0.064 | 0.170 | -0.013 |
| Ni | 3.337 | 0.170 | 1.989 | 0.170 |
| O | 0.170 | -0.013 | 0.170 | 0.064 |

TABLE S7: $SS_{AB}$, computed for the NiO **cell 2** with UHF.

| | Ni | O | Ni | O |
|---|---|---|---|---|
| Ni | 0.098 | 0.039 | 2.040 | 0.039 |
| O | 0.039 | -0.314 | 0.039 | 0.023 |
| Ni | 2.040 | 0.039 | 0.099 | 0.039 |
| O | 0.039 | 0.023 | 0.039 | -0.314 |

TABLE S8: $SS_{AB}$, computed for the NiO **cell 2** with GW.

| | Ni | O | Ni | O |
|---|---|---|---|---|
| Ni | 0.104 | 0.012 | 2.138 | 0.012 |
| O | 0.012 | -0.755 | 0.012 | 0.066 |
| Ni | 2.138 | 0.012 | 0.104 | 0.012 |
| O | 0.012 | 0.066 | 0.012 | -0.756 |

TABLE S9: $SS_{AB}^{\mathbf{k}=0}$, computed for the MnO **cell 1** with UHF.

| | Mn | O | Mn | O |
|---|---|---|---|---|
| Mn | -0.011 | 0.030 | 12.504 | 0.032 |
| O | 0.030 | 0.152 | 0.032 | 0.009 |
| Mn | 12.504 | 0.032 | -0.011 | 0.030 |
| O | 0.032 | 0.009 | 0.030 | 0.152 |

TABLE S10: $SS_{AB}^{\mathbf{k}=0}$, computed for the MnO **cell 1** with GW.

| | Mn | O | Mn | O |
|---|---|---|---|---|
| Mn | 0.035 | 0.157 | 12.841 | 0.148 |
| O | 0.157 | 0.300 | 0.148 | 0.021 |
| Mn | 12.841 | 0.148 | 0.035 | 0.157 |
| O | 0.148 | 0.021 | 0.157 | 0.300 |

TABLE S11: $SS_{AB}$, computed for the MnO **cell 1** with UHF.

| | Mn | O | Mn | O |
|---|---|---|---|---|
| Mn | -0.047 | 0.172 | 12.818 | 0.365 |
| O | 0.173 | -0.018 | 0.365 | 0.029 |
| Mn | 12.818 | 0.365 | -0.047 | 0.173 |
| O | 0.365 | 0.029 | 0.173 | -0.018 |

TABLE S12: $SS_{AB}$, computed for the MnO **cell 1** with GW.

| | Mn | O | Mn | O |
|---|---|---|---|---|
| Mn | 0.045 | 0.283 | 13.145 | 0.549 |
| O | 0.286 | 0.026 | 0.552 | 0.030 |
| Mn | 13.145 | 0.549 | 0.045 | 0.283 |
| O | 0.552 | 0.030 | 0.286 | 0.026 |

TABLE S13: $SS_{AB}^{\mathbf{k}=0}$, computed for the MnO **cell 2** with UHF.

| | Mn | O | Mn | O |
|---|---|---|---|---|
| Mn | 0.382 | 0.252 | 12.991 | 0.252 |
| O | 0.252 | 0.059 | 0.252 | 0.027 |
| Mn | 12.991 | 0.252 | 0.382 | 0.252 |
| O | 0.252 | 0.027 | 0.252 | 0.059 |

TABLE S14: $SS_{AB}^{\mathbf{k}=0}$, computed for the MnO **cell 2** with GW.

| | Mn | O | Mn | O |
|---|---|---|---|---|
| Mn | 0.807 | 0.341 | 13.294 | 0.341 |
| O | 0.341 | 0.134 | 0.341 | 0.059 |
| Mn | 13.294 | 0.341 | 0.807 | 0.341 |
| O | 0.341 | 0.059 | 0.341 | 0.134 |

TABLE S15: $SS_{AB}$, computed for the MnO **cell 2** with UHF.

| | Mn | O | Mn | O |
|---|---|---|---|---|
| Mn | 0.089 | 0.263 | 12.751 | 0.263 |
| O | 0.263 | 0.025 | 0.263 | 0.009 |
| Mn | 12.751 | 0.263 | 0.089 | 0.263 |
| O | 0.263 | 0.009 | 0.263 | 0.025 |

TABLE S16: $SS_{AB}$, computed for the MnO **cell 2** with GW.

| | Mn | O | Mn | O |
|---|---|---|---|---|
| Mn | 0.388 | 0.445 | 12.961 | 0.445 |
| O | 0.445 | 0.100 | 0.445 | 0.030 |
| Mn | 12.961 | 0.445 | 0.388 | 0.445 |
| O | 0.445 | 0.030 | 0.445 | 0.100 |

## 2. ENERGIES

TABLE S17: Total energies (a.u.), computed for the NiO **cell 1**.

| UHF | $2\times2\times2$ | $3\times3\times3$ | $4\times4\times4$ | $5\times5\times5$ |
|---|---|---|---|---|
| HS | -368.1628196 | -368.1461991 | -368.1386998 | -368.1357426 |
| BS | -367.8901924 | -368.1457511 | -368.1382406 | -368.1352836 |
| GW | $2\times2\times2$ | $3\times3\times3$ | $4\times4\times4$ | $5\times5\times5$ |
| HS | -369.2201592 | -369.2205394 | -369.2194387 | -369.2193687 |
| BS | -369.1570624 | -369.2196999 | -369.2184943 | -369.2184086 |

TABLE S18: Total energies (a.u.), computed for the NiO **cell 2**.

| UHF | $2\times2\times2$ | $3\times3\times3$ | $4\times4\times4$ | $5\times5\times5$ |
|---|---|---|---|---|
| HS | -368.1899809 | -368.1797182 | -368.1726283 | -368.1700018 |
| BS | -368.1932655 | -368.1816771 | -368.1744892 | -368.1718531 |
| GW | $2\times2\times2$ | $3\times3\times3$ | $4\times4\times4$ | $5\times5\times5$ |
| HS | -369.2504588 | -369.2537683 | -369.2528966 | -369.2531893 |
| BS | -369.2600060 | -369.2594930 | -369.2581984 | -369.2584717 |

TABLE S19: Extracted effective exchange couplings per f.u., K (meV), computed for NiO.

| UHF | $3\times3\times3$ | $4\times4\times4$ | $5\times5\times5$ |
|---|---|---|---|
| $J_{1,u}$ | 8.84 (0.762) | 9.06 (0.781) | 9.06 (0.781) |
| $J_{2,u}$ | -60.39 (-5.204) | -58.04 (-5.001) | -57.77 (-4.978) |
| GW | $3\times3\times3$ | $4\times4\times4$ | $5\times5\times5$ |
| $J_{1,u}$ | 16.57 (1.428) | 18.64 (1.606) | 18.95 (1.633) |
| $J_{2,u}$ | -167.21 (-14.409) | -158.15 (-13.628) | -157.96 (-13.611) |

TABLE S20: Total energies (a.u.), computed for the MnO **cell 1**.

| UHF | $2\times2\times2$ | $3\times3\times3$ | $4\times4\times4$ | $5\times5\times5$ |
|---|---|---|---|---|
| HS | -238.5037023 | -238.4890604 | -238.4826086 | -238.4800688 |
| BS | -238.5048633 | -238.4898538 | -238.4834350 | -238.4808944 |
| GW | $2\times2\times2$ | $3\times3\times3$ | $4\times4\times4$ | $5\times5\times5$ |
| HS | -239.5070981 | -239.5095263 | -239.5086973 | -239.5087988 |
| BS | -239.5100593 | -239.5117994 | -239.5110856 | -239.5111930 |

TABLE S21: Total energies (a.u.), computed for the MnO **cell 2**.

| UHF | $2 \times 2 \times 2$ | $3 \times 3 \times 3$ | $4 \times 4 \times 4$ | $5 \times 5 \times 5$ |
|---|---|---|---|---|
| HS | -238.5295077 | -238.5255375 | -238.5222547 | -238.5276638 |
| BS | -238.5335911 | -238.5268728 | -238.5233958 | -238.5287782 |
| GW | $2 \times 2 \times 2$ | $3 \times 3 \times 3$ | $4 \times 4 \times 4$ | $5 \times 5 \times 5$ |
| HS | -239.5315196 | -239.5453878 | -239.5479728 | -239.5564518 |
| BS | -239.5401971 | -239.5492329 | -239.5514149 | -239.5598399 |

TABLE S22: Extracted effective exchange couplings per f.u., K (meV), computed for MnO.

| UHF | $3 \times 3 \times 3$ | $4 \times 4 \times 4$ | $5 \times 5 \times 5$ |
|---|---|---|---|
| $J_{1,u}$ | -15.66 (-1.349) | -16.31 (-1.405) | -16.29 (-1.404) |
| $J_{2,u}$ | -19.48 (-1.679) | -13.72 (-1.182) | -13.03 (-1.123) |
| GW | $3 \times 3 \times 3$ | $4 \times 4 \times 4$ | $5 \times 5 \times 5$ |
| $J_{1,u}$ | -44.86 (-3.866) | -47.14 (-4.062) | -47.25 (-4.072 ) |
| $J_{2,}$ | -56.32 (-4.853) | -43.44 (-3.743) | -41.90 (-3.611) |
